# Supplementary material for: XNAS: Neural Architecture Search with Expert Advice
Source: arXiv:1906.08031 source file (2019-06-19)
Supplement: Supplementary file 1 [file XNAS_regret_proof.tex]

\label{XNAS_regret_proof}
\begin{proof}%[XNAS optimality]
\label{XNAS_optimality_proof}
We first state and prove $2$ additional auxiliary lemmas.
%We begin by stating and proving $3$ useful lemmas.
\begin{lemma}[Hoeffding] % \cite{cesa2006prediction}
\label{hoeffding}
For any random variable $X$ with $\Pr{\paren{a\leq X \leq b}}=1$ and $s\in \mathbb{R}$, %inequality
\begin{eqnarray}
  \ln{\Exp{e^{sX}}} \leq s\Exp{X} + \frac{s^2(b-a)^2}{8}.
\end{eqnarray}
\end{lemma}
Proof can be found in \cite{hoeffding1953lower}.
% \begin{lemma}
% \label{no_wipe}
% In XNAS, The optimal expert in hindsight cannot get wiped-out. 
% \end{lemma}
% The proof appears in \ref{sec:wipe_lemma_proof}.

\begin{lemma}
\label{sum_invariant}
The sum of unnormalized experts weights $V_t$ is invariant to Wipeout-and-Rescale.
\end{lemma}
\begin{proof}
By definition, $V_{t} = \sum_{i=1}^N v_{t,i}=v_{t-1,i}\cdot \exp{\{-\eta \nabla\ell_t (p_t)\cdot f_{t,i} \}}$. Summing the weights after wiping and rescaling:
\begin{eqnarray}
% v _{t-1,i}\cdot \exp{\{-\eta \nabla\ell_t (p_t)\cdot f_{t,i} \}} 
V'_t=\sum_{i=1}^N v _{t,i} \cdot \mathbbm{1}{(v _{t,i} \notag \geq   \theta)} \cdot \frac{V_t}{V_t-r_t} &=& \\ \notag
\frac{V_t}{V_t-r_t}  \sum_{i=1}^N v_{t,i} \paren{1-\mathbbm{1}{(v_{t,i} < \theta)}} &=& \\ \notag
\frac{V_t}{V_t-r_t}(V_t-r_t) &=& V_t.
\end{eqnarray}
\qed
\end{proof}
% let's define the sum of the unnormalized weights:
% \begin{eqnarray}
%   V_t&=&\sum_{i=1}^N v_{i,t}. \\
% \end{eqnarray}
Equipped with the above, we can get to the main proof.
We start with defining experts' auxiliary and accumulated-auxiliary losses following \cite{cesa2006prediction} ,
\begin{eqnarray}
\ell'_t(f_{t,i})&=& \nabla\ell (p_t)\cdot f_{t,i}= -R_{t,i} \\
%\end{eqnarray}
%Define the accumulated auxiliary loss of an expert,
%\begin{eqnarray}
L'_{T,i}&=&\sum_{t=1}^T \ell'_t(f_{t,i})
\end{eqnarray}
Notice that the auxiliary losses are bounded \ref{grad_bound}, $|\ell'_t(f_{t,i})| \leq \mathcal{L}$.
%\asaf{fix 2 refs, grad bound label and, wipe_rule}

We also define the set of non-wiped experts at time $t$,
\begin{eqnarray}
I_t=\braces{v_t|v_t>0}
\end{eqnarray}
We now bound the ratio of weights sums from both sides. For the lower bound:
\begin{eqnarray}
\ln{\frac{V_T}{V_0}}&=&\ln{\frac{\sum_{i=1}^N v_{T,i}}{N}} \notag\\
&=& \ln\paren{{\sum_{i\in I_T}\exp{\{-\eta L'_{T,i}}\}\cdot \gamma_t }} -\ln{N} \notag\\
&\geq& \ln{ \max_{i} \exp{\{-\eta L'_{T,i}}\}} +\ln{\frac{\gamma_T}{N}} \label{sum_to_max}  \\
&=&-\eta \min_{i}{L'_{T,i}} +\ln{\frac{\gamma_T}{N}}. \notag 
\end{eqnarray}

% \ln{\sum_{i=1}^N v_{T,i}} +\ln{\gamma_T} -\ln{N} \notag \\
% &=& \ln{\sum_{i=1}^N \exp{\{-\eta L'_{T,i}}\}}  +\ln{\frac{\gamma_T}{N}} \notag  \\
% &\geq& \ln{ \max_{i} \exp{\{-\eta L'_{T,i}}\}} +\ln{\frac{\gamma_T}{N}} \label{sum_to_max}  \\
% &=&-\eta \min_{i}{L'_{T,i}} +\ln{\frac{\gamma_T}{N}}. \notag 
% \end{eqnarray}
% \begin{eqnarray}
% \ln{\frac{V_T}{V_0}}&=&\ln{\sum_{i=1}^N v_{T,i}} +\ln{\gamma_T} -\ln{N} \notag \\
% &=& \ln{\sum_{i=1}^N \exp{\{-\eta L'_{T,i}}\}}  +\ln{\frac{\gamma_T}{N}} \notag  \\
% &\geq& \ln{ \max_{i} \exp{\{-\eta L'_{T,i}}\}} +\ln{\frac{\gamma_T}{N}} \label{sum_to_max}  \\
% &=&-\eta \min_{i}{L'_{T,i}} +\ln{\frac{\gamma_T}{N}}. \notag 
% \end{eqnarray}
Where we used lemma \ref{no_wipe} in \ref{sum_to_max}, assuring the existence of the loss minimizer among the non-wiped experts. Notice that since the wiped experts are always the ones with the smallest weights, their summed weight is equal or smaller then their fraction. For example, if in iteration $s$, $n_s$ experts were wiped out of $N_s$, 
\begin{eqnarray}
r_s \leq V_s \cdot \frac{n_s}{N_s}
\end{eqnarray}
Therefore,
\begin{eqnarray}
\frac{V_s}{V_s-r_s} \leq \frac{V_s}{V_s(1-\frac{n_s}{N_s})}=\frac{N_s}{N_s-n_s}
\end{eqnarray}
And the new number of experts is $N_{s+1}=N_s-n_s$. Therefore $\gamma_t$ can be upper bounded by the telescopic product term,
\begin{eqnarray}
\gamma_t = \prod_{s=1}^{t}\frac{V_s}{V_s-r_s} \leq \prod_{s=1}^{t} \frac{N_s}{N_s-n_s}=\prod_{s=1}^{t} \frac{N_s}{N_{s+1}}=\frac{N_1}{N_t}\leq \frac{N}{1}=N
\end{eqnarray}
Therefore $\forall{t}: \gamma_t \leq N$.\\
For the upper bound:
\begin{eqnarray}
\ln{\frac{V_t}{V_{t-1}}}&=&\ln{\frac{\sum_{i=1}^N  v_{t,i}}{\sum_{i=1}^N  v_{t-1,i}}} \notag \\ 
&=& \ln{ \frac{\sum_{i=1}^N  v_{t-1,i} \cdot \exp{\{-\eta \ell'_t(f_{t,i})\}}} {\sum_{i=1}^N  v_{t-1,i}}} \label{from_sum_invariant} \\ 
&\leq& -\eta \frac{\sum_{i=1}^N v_{t-1,i} \cdot \ell'_t(f_{t,i})}{\sum_{i=1}^N  v_{t-1,i}} + \frac{\eta^2 \mathcal{L}^2}{2} \label{from_hoef}\\
&=&   -\eta \ell'_t(p_t)  + \frac{\eta^2 \mathcal{L}^2}{2}. \label{aux_lin}
\end{eqnarray}
Where we used lemma \ref{sum_invariant} in \ref{from_sum_invariant}, and lemma \ref{hoeffding} in \ref{from_hoef}, with $a,b=\pm\mathcal{L}$. Equality \ref{aux_lin} is a result of the linearity of $\ell'_t$.

% The second inequality is due to the convexity of the loss function in its first parameter {todo: prove for l'-explain last inequality}.
% \ref{hoeffding} in the first inequality, 
% and lemma \ref{sum_invariant}  in the second one. 
% (refine: weights from wipeouted experts renormalize the survivals so we can work we the weights prior to the wipeout. Consider different letters in algo). \\
% In the last inequality we used the convexity of $\ell$ in its first parameter.
Summing the logs telescopic sum:
\begin{eqnarray*}
 \sum_{t=1}^T\ln{\frac{V_t}{V_{t-1}}} = \ln{\frac{V_T}{V_0}} \leq \sum_{t=1}^T  -\eta \ell'_t(p_t)  + \frac{\eta^2 T \mathcal{L}^2}{2}
\end{eqnarray*}

Combining the lower and upper bounds and dividing by $\eta$,
\begin{eqnarray}
\label{ell_bound}
\sum_{t=1}^T  \ell'_t(p_t)- \min_{i}{L'_{T,i}}  \leq \frac{\eta T\mathcal{L}^2}{2} +\frac{1}{\eta}\ln{\frac{\gamma_T}{N}} 
\end{eqnarray}

We now bound the accumulated regret, using the convexity of the loss,
\begin{eqnarray}
\mathrm{Regret}_T&=&\sum_{t=1}^T \ell_t(p_t) - \min_{i} \sum_{t=1}^T \ell_t({f_{t,i})} \notag \\
&=& \max_{i} \braces{\sum_{t=1}^T \ell_t (p_t) -\ell_t {(f_{t,i})}} \notag \notag \\
&\leq& \max_{i} \braces{\sum_{t=1}^T \nabla\ell_t(p_t) \cdot \paren{p_t-f_{t,i}}} \notag \\
&=& \max_{i} \braces{ \sum_{t=1}^T \ell'_t(p_t)-\ell'_t(f_{t,i})} \notag \\
&=& \sum_{t=1}^T  \ell'_t(p_t)- \min_{i}{L'_{T,i}}
\label{regret_ell_bound}
\end{eqnarray}

Combining \ref{ell_bound} and \ref{regret_ell_bound} completes the proof,
% From \ref{ell_bound} and \ref{regret_ell_bound} we have,
\begin{eqnarray}
\mathrm{Regret}_T \leq \frac{\eta T \mathcal{L}^2}{2} +\frac{1}{\eta}\ln N -\frac{1}{\eta}\ln{\gamma_T}
\end{eqnarray}
% % Ignoring the last term, picking the minimizer, $\eta=\sqrt{\frac{2\ln N}{T\mathcal{L}^2}}$, completes the proof.
% Picking the minimizer for the first two terms fully known in advance, $\eta=\sqrt{\frac{2\ln N}{T\mathcal{L}^2}}$, completes the proof.
%Ignoring the last term and picking the minimizer, 

% \begin{eqnarray}
% \mathrm{Regret}_T \leq \sqrt{2T\ln N}\mathcal{L} - \sqrt{\frac{T\mathcal{L}^2}{2\ln N}} \ln{\gamma_T}
% \end{eqnarray} 

% Dividing by $\eta$ and rearranging the terms,
% \begin{eqnarray}
% \mathrm{Regret}_T&=&\sum_{t=1}^T \ell_t(p_t) - \min_{i}{L_{T,i}} \\ &\leq& \frac{1}{\eta}\paren{\ln{N}- \sum_{i=1}^{T} \ln{\gamma_t}} + \frac{\eta T}{2} 
%   \\  &\leq&
%  \frac{1}{\eta}\ln{N} + \frac{\eta T}{2} .
% \end{eqnarray}
% Balancing the terms with *verify* $\eta=\sqrt{\frac{2\ln{N}}{T\mathcal{L}^2}}$ completes the proof.
% (todo: improve with a series $\eta_t$ according to $\ln{\gamma_t}$), or remove the term earlier. We can say that after every wipeout, $\eta$ can be decreased (small bound reduction when there are wipeouts.)
\qed
\end{proof}
% Explain that while in worst-case the term $\ln{\frac{W_t}{W_t-\mathrm{Regret}_T}}=0$, it's typically larger, resulting in smaller regret.
%TODO: add the gradient part, the Pi term + explanation.

% \begin{theorem}
% Cite corollary 2.5 from cesa or other source.
% \end{theorem}
