# Supplementary material for: XNAS: Neural Architecture Search with Expert Advice
Source: arXiv:1906.08031 source file (2019-06-19)
Supplement: Supplementary file 2 [file punch_line.tex]

DARTS \cite{liu2018darts} suggests a multiplicative update of the architecture weights altogether, by using gradient descent variant, e.g. ADAM \cite{kingma2014adam}, over variables that are driven through a softmax operation. This couples the update terms of different operations, attenuating the rewards received by weak operations, disallowing them to recover:
\begin{align} 
    \alpha_{t+1,i}= \alpha_{t,i} - \eta \partial_{\alpha_{t,i}}\ell_t(p_t) 
    \quad\longrightarrow\quad
    v_{t+1,i}= v_{t,i}e^{-\eta \nabla_{p_t}\ell_t(p_t) \cdot u_{t,i}\paren{f_{t,i}-p_t}}
\end{align} 
where, the transition is due to \eqref{eq:derivative_wrt_alpha} and \eqref{eq:forecaster}.
The corresponding reward is effectively $\tilde{R}_i = -\nabla_{p_t}\ell_t(p_t) \cdot u_{t,i}\paren{f_{t,i}-p_t}$.

SNAS \cite{xie2018snas} suggests to decouple the multiplicative updates of the weights by sampling paths, and shows that the corresponding effective reward is equivalent to $\tilde{R}_i = -\nabla_{p_t}\ell_t(p_t) \cdot f_{t,i}$. This indeed decouples the update terms of different operations, thus mitigates the attenuation of rewards, but in the cost of a substantial increase in runtime due to the sampling procedure.

By reviewing the problem as PEA setup, we suggest the XNAS algorithm, that corrects the attenuation occurs in $\tilde{R}_i$ by considering the decoupled reward $R_i$ while refraining from sampling paths.
