# Supplementary material for: XNAS: Neural Architecture Search with Expert Advice
Source: arXiv:1906.08031 source file (2019-06-19)
Supplement: Supplementary file 3 [file structure.tex]

--alternative representation of the paper's body (between intro and experiments).--
\\
Structure: (bullets are subsections)
\begin{enumerate}
    \item Introduction - Itamar / Lihi
    \item related work - Itamar / Lihi
    \item NAS space: - Itamar / Lihi (copy from previous paper).
    \begin{itemize}
        \item define mixedOp (+plot by niv without temperature).
        \item featuremap proagation equation and quick explanation of parent network.
        \item NAS optimization criterion and DARTS continuous relaxation. - Niv
        \item Definition of reward from SNAS theorem. - Niv
    \end{itemize}    
    \item Method:
    \begin{itemize}
        \item intro: NAS is a selection problem, not joint optimization- needs a tailor-made optimizer.
        \item present the algorithm, mention EG, SNAS reward, and discuss wipeout (speed, better convergence)
        \item consider: implementation is straightforward using softmax (will publish the optimizer?)
    \end{itemize}  
    \item Theoretical Analysis:
    \begin{itemize}
        \item We desire a worst-case optimizer as NAS is very non-stationary (alternate optimization).
        \item prediction with experts advice (define experts, regret)
        \item present main theorem (and the lemmas+lr selection), link to proof in supp. 
        \item Cite lower bound (discuss- worst case we achieve it, better cases we improve it due to wipeouts).
        \item Mention is scales better with many candidate operations (logN)
        \item Cite ADAM regret - $T*\sqrt{N}$ for worst-case
        \item Our theory suggest 2 (constant) learn-rates, with upper bound on size. A novel setup which we adopt.
    \end{itemize}
    \item Empirical Analysis
    \begin{itemize}
        \item intro: will discuss the learning process, focusing on a single mixedOp.
        \item subsubsection-Initialization bias: \\ SGD bad update (cite sharp+asap)+  2 toy models with deterministic and random setup showing a superior optimizer
        \item subsubsection-Topology optimization \\
        1. ADAM, used by all nas-algos, is heavy and has hyperparameters vs ours- lightweight with none. (maybe mention inside Initialization bias) \\
        2. bad practice: all algos treat arch-params as network params. It's a contest: regularization over arch-params is bad (entropy graph+connection to arbitrary cells and accuracy), lr should be large (mention our theoretic bound). \\
        3. Wipeout factor - control the search speed. \\
        5. Conclude: compare DARTS/SNAS to random-cell paper in terms of entropy (arbitrary selection) and results.
    \end{itemize}
    \item Experiments:
    \begin{itemize}
         \item Cifar-10 (search details + evaluation results)
             \item Transferability evaluation (Imagenet, additional datasets). Including comparison of the depth of cells in different NAS-algos (as part of the Transferability table\\
         \end{itemize}
         \item conclusion: - Itamar / Lihi
     \begin{itemize}
    \item The most unrandom NAS paper of all times. Basically repeating the contribution and strong points.
   
    \end{itemize}
\end{enumerate}
