# Supplementary material for: XNAS: Neural Architecture Search with Expert Advice
Source: arXiv:1906.08031 source file (2019-06-19)
Supplement: Supplementary file 4 [file todos.tex]

\begin{itemize}
    \item check that all refs/citations not broken.
    \item Abstract final touches.

    \item Consider moving the weight-decay graph to the appendix and relate in body.
    \item Full read by members and fixes.
    \item Bold for all tensors/vectors.
    \item shrink the lr paragraph based on what written in 'theory'.
    \item headlines - All Like That. 
    \item Move the 'wipeout' subsection from the 'Few Hyper Parameters' section
    \item consistent reference to sections/figures/algorithms/supplementary material (capital letters or not, '-' or not)
    \item reorder supp sections.
    \item Elaborate on the mean normalized entropy calculations in the supp !!!!
    \item consider uniting the supp mentions in late bloomers.
\end{itemize}

\textbf{DONE}
\begin{itemize}
\item Decide on the way we relate to stuff in the supplementary (simulation, details)- done.
    \item Reorder figs/tables better. - done
    \item Change title and abstract in the cmt upload. - done
    \item Upload first version. - done.
    \item Naming- pass and correct (e.g. predictor/mixedop->forecaster)-done
    \item Decide on which sections enters the paper. - done
    \item (deal and) remove all comments. -done.
    \item Detailed Experiments Setting: edit sections (done).
    \item sections changes (old methodology) based on Lihi's suggestions. (done)
    \item Check for corrupted/duplicated bibliography (tal-done, no warnings)
    \item Discuss 3 mentioning of darts - Asaf -done
        \item A careful read by a native speaker + fixes. - done
    \item Wipeout- decide on the graph/elaboration. -done
    \item lose bound-> reward bound in algorithm1.-done
    \item Consider changing the bound L to R, as it bound the update reward and not a loss. - done (no change)
    \item align: wipe-out, wipeout.-done
    \item Break proof according to theory part and link. - done
    \item Fix compilation errors (possibly affecting the structure).-done
    \item Add 'For brevity, supplementary'-done
    \item delete the 'punch line' section in the supp - done
    \item Order of indices of time and expert: $L_{s,i}$
    \item Many changes in notations, algo (Yonathan) and proof (notations).
\end{itemize}
