# Supplementary material for: XNAS: Neural Architecture Search with Expert Advice
Source: arXiv:1906.08031 source file (2019-06-19)
Supplement: Supplementary file 5 [file wipe_lemma_proof.tex]

% \begin{lemma}
% \label{no_wipe}
% In XNAS, The optimal expert in hindsight cannot get wiped-out. 
% \end{lemma}
\label{sec:wipe_lemma_proof}
\begin{proof}
% Since the updates are bounded, so are the ratios between weights..... 
By contradiction, assume that expert $j$ is being wiped-out at iteration $t$ based on \ref{wipe_rule}, and without loss of generality, $k\neq j$ is the leading expert at that time,
% The condition for for expert $j$ being wiped-out at iteration $t$,
\begin{eqnarray} \label{contra}
v_{t,k} &=& \arg\max_{i}\{v_{t,i}\} \notag \\
v_{t,j}&<&v_{t,k} \cdot \exp{\{-2\eta\mathcal{L}(T-t)\}} 
% \\
% v_{T,j}&=&\max_{i}\{v_{T,i}\}
\end{eqnarray}
Since expert $j$ is the optimal one in hindsight, specifically, 
\begin{eqnarray} 
\label{contra_hind}
%v_{T,j} &=& \arg\max_{i}\{v_{T,i}\}
v_{T,j} \geq v_{T,k}
% v_{t,j}&<&\max_{i}\{v_{t,i}\} \cdot \exp{\{-2\eta\mathcal{L}(T-t)\}} \\
% v_{T,j}&=&\max_{i}\{v_{T,i}\}
\end{eqnarray}
However, since the loss is $\mathcal{L}$-bounded, the ratios between weights at time $t,T$ are bounded as well,
\begin{eqnarray} 
v_{T,k} &\geq& v_{t,k} \cdot \exp{\{-\eta\mathcal{L}(T-t)\}}\cdot\frac{\gamma_T}{\gamma_t}\\
v_{T,j} &\leq& v_{t,j} \cdot \exp{\{\eta\mathcal{L}(T-t)\}} \cdot \frac{\gamma_T}{\gamma_t}
\label{contra_bounded}
\end{eqnarray}
% In order to get wiped-out, an expert's weight should,
Where $\gamma_T \gamma_t^{-1}$ is the aggregated rescale between iterations $t,..,T$. Recap inequalities \ref{contra_hind}-\ref{contra_bounded},
\begin{eqnarray*}
v_{t,j} &\geq&  v_{T,j}\cdot\exp{\{-\eta\mathcal{L}(T-t)\}} \cdot \paren{\frac{\gamma_t}{\gamma_T}}^{-1} \notag \\ &\geq&  v_{T,k}\cdot\exp{\{-\eta\mathcal{L}(T-t)\}} \cdot \paren{\frac{\gamma_t}{\gamma_T}}^{-1}  \notag \\ &\geq&  v_{t,k}\cdot\exp{\{-2\eta\mathcal{L}(T-t)\}}\cdot 1
\end{eqnarray*}
In contradiction to \ref{contra}.
\qed
\end{proof}
