# Supplementary material for: XNAS: Neural Architecture Search with Expert Advice
Source: arXiv:1906.08031 source file (2019-06-19)
Supplement: Supplementary file 6 [file XNAS_reget_proof_new.tex]

\label{XNAS_regret_proof}
\begin{proof}%[XNAS optimality]
%\label{XNAS_optimality_proof}
We first state and prove  $3$ useful lemmas.
%We begin by stating and proving $3$ useful lemmas.
\begin{lemma}[Hoeffding] % \cite{cesa2006prediction}
\label{hoeffding}
For any random variable $X$ with $\Pr{\paren{a\leq X \leq b}}=1$ and $s\in \mathbb{R}$, %inequality
\begin{eqnarray}
  \ln{\Exp{e^{sX}}} \leq s\Exp{X} + \frac{s^2(b-a)^2}{8}.
\end{eqnarray}
\end{lemma}
Proof can be found in \cite{hoeffding1953lower}.
\begin{lemma}
\label{no_wipe}
In XNAS, The optimal expert in hindsight cannot get wiped-out. 
\end{lemma}
\begin{proof}
% Since the updates are bounded, so are the ratios between weights..... 
By contradiction, assume that expert $j$ is being wiped-out at iteration $t$ based on \ref{wipe_rule}, and without loss of generality, $k\neq j$ is the leading expert at that time,
% The condition for for expert $j$ being wiped-out at iteration $t$,
\begin{eqnarray} \label{contra}
v_{t,k} &=& \arg\max_{i}\{v_{t,i}\} \notag \\
v_{t,j}&<&v_{t,k} \cdot \exp{\{-2\eta\mathcal{L}(T-t)\}} 
% \\
% v_{T,j}&=&\max_{i}\{v_{T,i}\}
\end{eqnarray}
Since expert $j$ is the optimal one in hindsight, specifically, 
\begin{eqnarray} 
\label{contra_hind}
%v_{T,j} &=& \arg\max_{i}\{v_{T,i}\}
v_{T,j} \geq v_{T,k}
% v_{t,j}&<&\max_{i}\{v_{t,i}\} \cdot \exp{\{-2\eta\mathcal{L}(T-t)\}} \\
% v_{T,j}&=&\max_{i}\{v_{T,i}\}
\end{eqnarray}
However, since the loss is $\mathcal{L}$-bounded, the ratios between weights at time $t,T$ are bounded as well,
\begin{eqnarray} 
v_{T,k} &\geq& v_{t,k} \cdot \exp{\{-\eta\mathcal{L}(T-t)\}} \\
v_{T,j} &\leq& v_{t,j} \cdot \exp{\{\eta\mathcal{L}(T-t)\}} 
\label{contra_bounded}
\end{eqnarray}
% In order to get wiped-out, an expert's weight should,
Recap inequalities \ref{contra_hind}-\ref{contra_bounded},
\begin{eqnarray*}
v_{t,j} &\geq&  v_{T,j}\cdot\exp{\{-\eta\mathcal{L}(T-t)\}} \notag \\ &\geq&  v_{T,k}\cdot\exp{\{-\eta\mathcal{L}(T-t)\}} \notag \\ &\geq&  v_{t,k}\cdot\exp{\{-2\eta\mathcal{L}(T-t)\}}
\end{eqnarray*}
In contradiction to \ref{contra}.
\qed
\end{proof}

\begin{lemma}
\label{sum_invariant}
The sum of unnormalized experts weights $V_t$ is invariant to Wipeout-and-Rescale.
\end{lemma}
\begin{proof}
By definition, $V_{t} = \sum_{i=1}^N v_{t,i}=v_{t-1,i}\cdot \exp{\{-\eta \nabla\ell (\hat{y_t},y_t)\cdot f_{t,i} \}}$. Summing the weights after wiping and rescaling:
\begin{eqnarray}
% v _{t-1,i}\cdot \exp{\{-\eta \nabla\ell (\hat{y_t},y_t)\cdot f_{t,i} \}} 
\sum_{i=1}^N v _{t,i} \cdot \mathbbm{1}{(v _{t,i} \notag \geq   \Theta)} \cdot \frac{V_t}{V_t-r_t} &=& \\ \notag
\frac{V_t}{V_t-r_t}  \sum_{i=1}^N v_{t,i} \paren{1-\mathbbm{1}{(v_{t,i} < \Theta)}} &=& \\ \notag
\frac{V_t}{V_t-r_t}(V_t-r_t) &=& V_t.
\end{eqnarray}
\qed
\end{proof}
% let's define the sum of the unnormalized weights:
% \begin{eqnarray}
%   V_t&=&\sum_{i=1}^N v_{i,t}. \\
% \end{eqnarray}
Equipped with the above, we can get to the main proof.
We start with defining experts' auxiliary and accumulated-auxiliary losses following \cite{cesa2006prediction} ,
\begin{eqnarray}
\ell'(f_{t,i})&=& \nabla\ell (\hat{y_t},y_t)\cdot f_{t,i} \\
%\end{eqnarray}
%Define the accumulated auxiliary loss of an expert,
%\begin{eqnarray}
L'_{T,i}&=&\sum_{t=1}^T \ell'(f_{t,i})
\end{eqnarray}
Notice that the auxiliary losses are bounded \ref{grad_bound}, $\ell'_{t,i} \leq \mathcal{L}$.
%\asaf{fix 2 refs, grad bound label and, wipe_rule}
We Now bound the ratio of weights sums from both sides. For the lower bound:
\begin{eqnarray}
\ln{\frac{V_T}{V_0}}&=&\ln{\sum_{i=1}^N v_{T,i}} +\ln{\gamma_T} -\ln{N} \notag \\
&=& \ln{\sum_{i=1}^N \exp{\{-\eta L'_{T,i}}\}}  +\ln{\frac{\gamma_T}{N}} \notag  \\
&\geq& \ln{ \max_{i} \exp{\{-\eta L'_{T,i}}\}} +\ln{\frac{\gamma_T}{N}} \label{sum_to_max}  \\
&=&-\eta \min_{i}{L'_{T,i}} +\ln{\frac{\gamma_T}{N}}. \notag 
\end{eqnarray}
Where we used lemma \ref{no_wipe} in \ref{sum_to_max}, assuring the existence of the loss minimizer among the non-wiped experts. 
For the upper bound:
\begin{eqnarray}
\ln{\frac{V_t}{V_{t-1}}}&=&\ln{\frac{\sum_{i=1}^N  v_{t,i}}{\sum_{i=1}^N  v_{t-1,i}}} \notag \\ 
&=& \ln{ \frac{\sum_{i=1}^N  v_{t-1,i} \cdot \exp{\{-\eta \ell'(f_{t,i})\}}} {\sum_{i=1}^N  v_{t-1,i}}} \label{from_sum_invariant} \\ 
&\leq& -\eta \frac{\sum_{i=1}^N v_{t-1,i} \cdot \ell'(f_{t,i})}{\sum_{i=1}^N  v_{t-1,i}} + \frac{\eta^2 \mathcal{L}^2}{2} \label{from_hoef}\\
&=&   -\eta \ell'(\hat{y_t})  + \frac{\eta^2 \mathcal{L}^2}{2}. \label{aux_lin}
\end{eqnarray}
Where we used lemma \ref{sum_invariant} in \ref{from_sum_invariant}, and lemma \ref{hoeffding} in \ref{from_hoef}, with $a,b=\pm\mathcal{L}$. Equality \ref{aux_lin} is a result of $\ell'$ linearity.

% The second inequality is due to the convexity of the losS function in its first parameter {todo: prove for l'-explain last inequality}.
% \ref{hoeffding} in the first inequality, 
% and lemma \ref{sum_invariant}  in the second one. 
% (refine: weights from wipeouted experts renormalize the survivals so we can work we the weights prior to the wipeout. Consider different letters in algo). \\
% In the last inequality we used the convexity of $\ell$ in its first parameter.
Summing the logs telescopic sum:
\begin{eqnarray*}
 \sum_{t=1}^T\ln{\frac{V_t}{V_{t-1}}} = \ln{\frac{V_T}{V_0}} \leq \sum_{t=1}^T  -\eta \ell'(\hat{y_t})  + \frac{\eta^2 T \mathcal{L}^2}{2}
\end{eqnarray*}

Combining the lower and upper bounds and dividing by $\eta$,
\begin{eqnarray}
\label{ell_bound}
\sum_{t=1}^T  \ell'(\hat{y_t})- \min_{i}{L'_{T,i}}  \leq \frac{\eta T\mathcal{L}^2}{2} +\frac{1}{\eta}\ln{\frac{\gamma_T}{N}} 
\end{eqnarray}

We now bound the accumulated regret, using the convexity of the loss in its first argument,
\begin{eqnarray}
R_T&=&\sum_{t=1}^T \ell (\hat{y_t},y_t) - \min_{i} \sum_{t=1}^T \ell ({f_{t,i},y_t)} \notag \\
&=& \max_{i} \braces{\sum_{t=1}^T \ell (\hat{y_t},y_t) -\ell {(f_{t,i},y_t)}} \notag \notag \\
&\leq& \max_{i} \braces{\sum_{t=1}^T \nabla\ell (\hat{y_t},y_t) \cdot \paren{\hat{y_t}-f_{t,i}}} \notag \\
&=& \max_{i} \braces{ \sum_{t=1}^T \ell'(\hat{y_t})-\ell'(f_{t,i})} \notag \\
&=& \sum_{t=1}^T  \ell'(\hat{y_t})- \min_{i}{L'_{T,i}}
\label{regret_ell_bound}
\end{eqnarray}

From \ref{ell_bound} and \ref{regret_ell_bound} we have,
\begin{eqnarray}
R_T \leq \frac{\eta T \mathcal{L}^2}{2} +\frac{1}{\eta}\ln N -\frac{1}{\eta}\ln{\gamma_T}
\end{eqnarray}
% Ignoring the last term, picking the minimizer, $\eta=\sqrt{\frac{2\ln N}{T\mathcal{L}^2}}$, completes the proof.
Picking the minimizer for the first two terms fully known in advance, $\eta=\sqrt{\frac{2\ln N}{T\mathcal{L}^2}}$, completes the proof.
%Ignoring the last term and picking the minimizer, 

% \begin{eqnarray}
% R_T \leq \sqrt{2T\ln N}\mathcal{L} - \sqrt{\frac{T\mathcal{L}^2}{2\ln N}} \ln{\gamma_T}
% \end{eqnarray} 

% Dividing by $\eta$ and rearranging the terms,
% \begin{eqnarray}
% R_T&=&\sum_{t=1}^T \ell(\hat{y_t},y_t) - \min_{i}{L_{T,i}} \\ &\leq& \frac{1}{\eta}\paren{\ln{N}- \sum_{i=1}^{T} \ln{\gamma_t}} + \frac{\eta T}{2} 
%   \\  &\leq&
%  \frac{1}{\eta}\ln{N} + \frac{\eta T}{2} .
% \end{eqnarray}
% Balancing the terms with *verify* $\eta=\sqrt{\frac{2\ln{N}}{T\mathcal{L}^2}}$ completes the proof.
% (todo: improve with a series $\eta_t$ according to $\ln{\gamma_t}$), or remove the term earlier. We can say that after every wipeout, $\eta$ can be decreased (small bound reduction when there are wipeouts.)
\qed
\end{proof}
% Explain that while in worst-case the term $\ln{\frac{W_t}{W_t-r_t}}=0$, it's typically larger, resulting in smaller regret.
%TODO: add the gradient part, the Pi term + explanation.

% \begin{theorem}
% Cite corollary 2.5 from cesa or other source.
% \end{theorem}
